# Supplementary material for: Tonal consonance parameters link microscopic and macroscopic properties of music exposing a hidden order in melody
Source: arXiv:1610.04551 ancillary file (2017-04-23)
Supplement: Supplementary file 1 [file Supplementary_Material.pdf]

# Supplementary material

## Superposition of two pure tones with different amplitudes and phases

The superposition $x(t)$ of two pure tones with different amplitudes ($A_1$ and $A_2$), different phases ($\varphi_1$ and $\varphi_2$), and different frequencies ($f_1 = \omega_1/2\pi$ and $f_2 = \omega_2/2\pi$), where $\omega_i$ is an angular frequency, is given by

$$x(t) = x_1(t) + x_2(t) = A_1 \cos(\omega_1 t + \varphi_1) + A_2 \cos(\omega_2 t + \varphi_2)$$

where $t$ is the time. Defining

$$\omega_+ = \frac{\omega_1 + \omega_2}{2} \ ; \ \varphi_+ = \frac{\varphi_1 + \varphi_2}{2} \ ; \ \omega_- = \frac{\omega_1 - \omega_2}{2} \ ; \ \varphi_- = \frac{\varphi_1 + \varphi_2}{2}$$

then

$$x(t) = (A_1 + A_2)cos(\omega_+ t + \varphi_+)cos(\omega_- t + \varphi_-) + (A_2 - A_1)sin(\omega_+ t + \varphi_+)sin(\omega_- t + \varphi_-)$$

This equation indicates that the frequency of the oscillations in time only depends on $\omega_+$ and $\omega_-$, independently of phases and amplitudes. Since $\omega = 2\pi f$ then the frequency of oscillations is given by the sum and the difference of the frequencies $f_1$ and $f_2$. In the case of sound waves, for $|f_1 - f_2| \leq 20\, Hz$ with $|f_1 - f_2| \ll f_1 + f_2$, people hear a tone of frequency $f_R = (f_1 + f_2)/2$ with beats (shocks waves produced by fluctuations in the peak intensity) at the frequency $f_B = |f_1 - f_2|$. This phenomenon can be appreciated by plotting $x$ as a function of $t$ and counting the number of rapid oscillations and peaks in the amplitude per unit of time.

## The lowest fundamental frequency of a pair of complex tones is a parameter equivalent to the absolute value of the difference between the fundamental frequencies, when the ratio between the fundamental frequencies is assumed to be constant

Reinier Plomp and Willem Levelt parameterized the consonance level of pairs of complex tones using the relation between tonal consonance and the fundamental frequency of the lowest tone for musical intervals of equal size. Using the fact that for the fundamental frequencies of a pair of complex tones the interval relation $f_j = \alpha_{(j-i)} \cdot f_i$, with $\alpha_{(j-i)}$ determined by the size of the interval $j - i$ for a specific musical scale, the frequency difference $f_j - f_i$ can be written as $f_j - f_i = f_i(\alpha_{(j-i)} - 1)$. Since $\alpha_{(j-i)} - 1$ is constant for intervals of equal size, then tonal consonance and the difference of the fundamental frequencies have the same functional relation.

## Tonal consonance of complex tones: Intervals of equal size played in different locations within the register

*Step one: Tonal consonance associated with a timbre:*
For the superposition of two pure tones of frequencies $f_1$ and $f_2$ ($f_1 < f_2$) with amplitudes $a_1$ and $a_2$ respectively, William Sethares measured the level of dissonance parameterizing the Plomp and Levelt curves using a mathematical function given by:

$$d(f_1, f_2, a_1, a_2) = (a_1)(a_2)\left[e^{-b_1 s(f_2 - f_1)} - e^{-b_2 s(f_2 - f_1)}\right] ,$$

where $b_1 = 3.5$ ; $b_2 = 5.75$ ; $s = \frac{0.24}{(0.021)(f_1)+19}$ .
In this last equation we can appreciate that smaller amplitudes contribute less than larger ones.
For a complex tone with $n$ partials, the total dissonance $D_F$ can be calculated by superposing the individual dissonances corresponding to each possible pair of partials, that is:

$$D_F = \frac{1}{2}\sum_{i=1}^{n}\sum_{j=1}^{n} d\left(f_i, f_j, a_i, a_j\right) .$$

*Step two: Tonal consonance associated with pairs of complex tones played with the same timbre:*
If we superpose two different complex tones with the same timbre and with a ratio of fundamental frequencies of $f_j/f_i = \alpha$, with ($f_j > f_i$), the total dissonance of this superposition $D_F(\alpha)$ is given by:

$$D_F(\alpha) = D_F + D_{\alpha F} + \sum_{i=1}^{n}\sum_{j=1}^{n} d\left(f_i, \alpha f_j, a_i, a_j\right),$$

where $D_F$ and $D_{\alpha F}$ correspond to the total dissonance associated with the timbre of each complex tone, and the last term corresponds to the total dissonance generated by the interaction between the partials of the two complex tones.
In this last equation, we have supposed that for a given timbre the amplitudes and the relative space between the partials in the spectrum are the same, independently of the fundamental frequency.

*Step three: Tonal consonance associated with a particular musical interval (with a particular timbre) played in different parts of the register:*
In order to understand the dependence between the tonal consonance (for a particular frequency ratio) and the fundamental frequency $f_1$ present in the "$s$" parameter of the first equation presented in the section "Tonal consonance associated with a timbre", we fixed the quantity $\alpha$ and then we varied the value of the frequency $f_1$. This is equivalent to fixing a particular interval size in semitones and transposing this interval to different parts of the register of a musical instrument. Replicating this procedure for different values of $\alpha$, it is possible to generate the tonal consonance curves for complex tones in different parts of the register for all the particular ratios present in a musical scale.

# Frequency ratios used to construct the Pythagorean, just, and twelve-tone equal-tempered scales

| | Just scale | | | Pythagorean scale | | | Tempered scale |
|---|---|---|---|---|---|---|---|
| Interval size (semitones) | *n* | *m* | *n/m* | *n* | *m* | *n/m* | $f_j/f_i$ |
| 0 | 1 | 1 | 1.000 | 1 | 1 | 1.000 | 1 |
| 1 | 16 | 15 | 1.067 | 2187 | 2048 | 1.068 | $2^{(1/12)}$ |
| 2 | 9 | 8 | 1.125 | 9 | 8 | 1.125 | $2^{(2/12)}$ |
| 3 | 6 | 5 | 1.200 | 32 | 27 | 1.185 | $2^{(3/12)}$ |
| 4 | 5 | 4 | 1.250 | 81 | 64 | 1.266 | $2^{(4/12)}$ |
| 5 | 4 | 3 | 1.333 | 4 | 3 | 1.333 | $2^{(5/12)}$ |
| 6 | 45 | 32 | 1.406 | 729 | 512 | 1.424 | $2^{(6/12)}$ |
| 7 | 3 | 2 | 1.500 | 3 | 2 | 1.500 | $2^{(7/12)}$ |
| 8 | 8 | 5 | 1.600 | 6561 | 4096 | 1.602 | $2^{(8/12)}$ |
| 9 | 5 | 3 | 1.667 | 27 | 16 | 1.688 | $2^{(9/12)}$ |
| 10 | 16 | 9 | 1.778 | 16 | 9 | 1.778 | $2^{(10/12)}$ |
| 11 | 15 | 8 | 1.875 | 243 | 128 | 1.898 | $2^{(11/12)}$ |
| 12 | 2 | 1 | 2.000 | 2 | 1 | 2.000 | 2 |

**Supplementary Table 1. Coefficients for generating the Pythagorean, just, and twelve-tone equal-tempered scales.** Interval size up to one octave (12 semitones).

# Unique values for the quantities $f_j - f_i$ and $f_i^2 - f_j^2$ in the Pythagorean, just and twelve-tone equal-tempered scales

We use three musical scales: Pythagorean, just, and Twelve-Tone Equal-Tempered. For each of these scales, we consider the consequences of degenerated values $f_j^2 - f_i^2 = f_n^2 - f_m^2$, except for unisons ($i = j$, $m = n$), where $i \neq m$ and $j \neq n$. This equality holds for the following conditions: $f_j > f_i$ and $f_n > f_m$ for ascending transitions or $f_j < f_i$ and $f_n < f_m$ for descending transitions. Since for descending transitions $f_i^2 - f_j^2 = f_m^2 - f_n^2$ the difference between the cases of ascending and descending transitions is just the order of the subindices, we analyze the case of ascending transitions without loss of generality.

For each scale we can express $f_j = \alpha_{(j-i)} \cdot f_i$ and $f_n = \alpha_{(n-m)} \cdot f_m$, then $f_i^2[\alpha_{(j-i)}^2 - 1] = f_m^2[\alpha_{(n-m)}^2 - 1]$ or

$$\frac{f_i^2}{f_m^2} = \frac{[\alpha_{(n-m)}^2 - 1]}{[\alpha_{(j-i)}^2 - 1]}.$$

For $> m$ then $f_i^2/f_m^2 = \alpha_{(i-m)}^2$ and for $i < m$ $f_i^2/f_m^2 = 1/\alpha_{(i-m)}^2$ .

Finally, the degeneracy equations are

$$\frac{[\alpha_{(n-m)}^2 - 1]}{[\alpha_{(j-i)}^2 - 1]} = \alpha_{(i-m)}^2 \text{ for } i > m \text{ and } \frac{[\alpha_{(n-m)}^2 - 1]}{[\alpha_{(j-i)}^2 - 1]} = \frac{1}{\alpha_{(i-m)}^2} \text{ for } i < m.$$

We also use this procedure to obtain the degeneracy equations for the difference of frequencies $f_j - f_i = f_n - f_m$

$$\frac{[\alpha_{(n-m)} - 1]}{[\alpha_{(j-i)} - 1]} = \alpha_{(i-m)} \text{ for } i > m \text{ and } \frac{[\alpha_{(n-m)} - 1]}{[\alpha_{(j-i)} - 1]} = \frac{1}{\alpha_{(i-m)}} \text{ for } i < m.$$

We generate all possible combinations of the coefficients $\alpha_{(n-m)}$ to find the number of times that the degeneracy equations are satisfied, which depends on the precision in the decimal places. Supplementary Figure 1 shows the percentage of times that the degeneracy equations are satisfied, over a total range of $87 \times 87 \times 87 = 658503$ possibilities (corresponding to an 88-pitch musical instrument such as an 88-key piano), as a function of the precision (measured in decimal places) used to calculate the left and the right part of the degeneracy equations. The values of α for the Pythagorean, just, and twelve-tone equal-tempered scales are calculated from the values $n/m$ and $f_j/f_i$ presented in Supplementary Table 1. For all scales, the α coefficients corresponding to intervals larger than one octave are obtained by multiplying the corresponding coefficient of the previous octave by 2. In our algorithm, the degeneracy equations are satisfied when the absolute value of the difference between the left and the right parts of each equation is less than $1 \times 10^{-15}$.

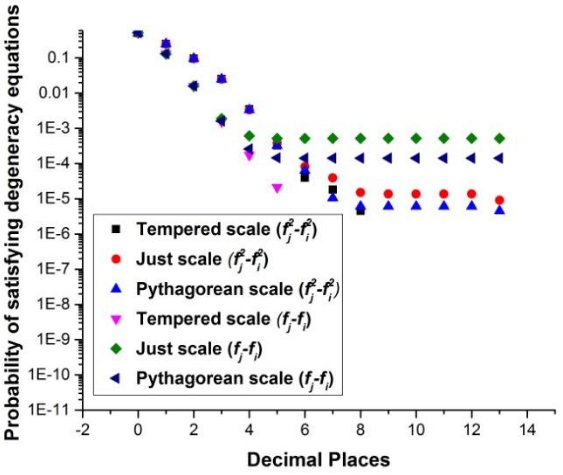


**Supplementary Figure 1. Probability of satisfying the degeneracy equations vs. decimal places used to calculated the degeneracy equations.** The figure shows the probability of satisfying the degeneracy equations in the case of an 88-pitch instrument for the quantities $f_j^2 - f_i^2$ and $f_j - f_i$ in three different scales: Twelve-Tone Equal-Tempered, just, and Pythagorean. For the twelve-tone equal-tempered scale, the degeneracy equations are not satisfied beyond 5 decimal places for $f_j - f_i$ and beyond 8 decimal places for $f_j^2 - f_i^2$. For the just and the Pythagorean scales, and using 13 decimal places, the number of times that the degeneracy equations are satisfied for the quantity $f_j^2 - f_i^2$ reduces to 7 and 3, respectively (corresponding to an order of magnitude of 1E-5 in the probability). However, for the quantity $f_j - f_i$, the number of times that the degeneracy equations are satisfied reduces to 341 and 92, respectively (corresponding to an order of magnitude of 1E-3 in the probability). In our algorithm, the degeneracy equations are satisfied when the absolute value of the difference between the left and the right part of each equations is less than $1 \times 10^{-15}$.

## Determination coefficients $R^2$ for the fit to an exponential function in the CCDF and histograms, for the case of the quantities $|f_j - f_i|$ and $|f_j^2 - f_i^2|$

| | | CCDF | | | | | | Histograms | | | | | |
|---|---|---|---|---|---|---|---|---|---|---|---|---|---|
| | | $\|f_{(i+1)}-f_{(i)}\|$ | $\|f_{(i+1)}^2-f_{(i)}^2\|$ | $\|f_{(i+1)}-f_{(i)}\|+$ | $\|f_{(i+1)}-f_{(i)}\|-$ | $\|f_{(i+1)}^2-f_{(i)}^2\|+$ | $\|f_{(i+1)}^2-f_{(i)}^2\|-$ | $\|f_{(i+1)}-f_{(i)}\|$ | $\|f_{(i+1)}^2-f_{(i)}^2\|$ | $\|f_{(i+1)}-f_{(i)}\|+$ | $\|f_{(i+1)}-f_{(i)}\|-$ | $\|f_{(i+1)}^2-f_{(i)}^2\|+$ | $\|f_{(i+1)}^2-f_{(i)}^2\|-$ |
| Third Brandenbug Concerto | Violin 1 | 0.99613 | 0.99719 | 0.99822 | 0.99482 | 0.99549 | 0.99532 | 0.97461 | 0.99671 | 0.99771 | 0.96960 | 0.99860 | 0.99050 |
| | Violin 2 | 0.99720 | 0.99522 | 0.99682 | 0.99183 | 0.99357 | 0.98828 | 0.99202 | 0.99738 | 0.99497 | 0.99419 | 0.98618 | 0.99115 |
| | Violin 3 | 0.99826 | 0.99458 | 0.99590 | 0.99296 | 0.99122 | 0.98703 | 0.99588 | 0.98979 | 0.99870 | 0.99663 | 0.99138 | 0.99695 |
| | Viola 1 | 0.99690 | 0.99616 | 0.99339 | 0.99146 | 0.98750 | 0.98683 | 0.98058 | 0.97628 | 0.98559 | 0.99433 | 0.97761 | 0.99361 |
| | Viola 2 | 0.99572 | 0.99312 | 0.98949 | 0.98226 | 0.98216 | 0.97975 | 0.98669 | 0.98637 | 0.97808 | 0.99513 | 0.98102 | 0.99427 |
| | Viola 3 | 0.99589 | 0.99277 | 0.98768 | 0.98067 | 0.98114 | 0.97855 | 0.99322 | 0.98978 | 0.97801 | 0.99527 | 0.98090 | 0.99612 |
| | Cello 1 | 0.98868 | 0.99195 | 0.99468 | 0.98246 | 0.99126 | 0.98999 | 0.99376 | 0.99218 | 0.99733 | 0.99322 | 0.99147 | 0.99721 |
| | Cello 2 | 0.98887 | 0.99223 | 0.99488 | 0.98284 | 0.99147 | 0.99035 | 0.99365 | 0.99235 | 0.99736 | 0.99381 | 0.99181 | 0.99745 |
| | Cello 3 | 0.98832 | 0.99142 | 0.99466 | 0.98192 | 0.99132 | 0.98876 | 0.99364 | 0.99678 | 0.99783 | 0.99265 | 0.99236 | 0.99711 |
| | Violone | 0.98718 | 0.99079 | 0.99307 | 0.97590 | 0.98629 | 0.98348 | 0.99226 | 0.99089 | 0.99587 | 0.99295 | 0.98961 | 0.99661 |
| | Harpsichord | 0.98718 | 0.99079 | 0.99307 | 0.97590 | 0.98629 | 0.98348 | 0.99226 | 0.99089 | 0.99587 | 0.99404 | 0.98961 | 0.99661 |
| Missa Dixit Maria | Soprano | 0.96450 | 0.97219 | 0.99292 | 0.97157 | 0.98935 | 0.97597 | 0.80746 | 0.79343 | 0.99230 | 0.83315 | 0.96212 | 0.95440 |
| | Contralto | 0.96977 | 0.98016 | 0.98716 | 0.97415 | 0.98414 | 0.98051 | 0.94996 | 0.96966 | 0.99846 | 0.92906 | 0.99367 | 0.94612 |
| | Tenor | 0.97258 | 0.97930 | 0.99171 | 0.98456 | 0.99114 | 0.99017 | 0.88303 | 0.95319 | 0.99527 | 0.95344 | 0.97790 | 0.97827 |
| | Bass | 0.98360 | 0.99073 | 0.98565 | 0.98553 | 0.98849 | 0.98765 | 0.84540 | 0.86061 | 0.93378 | 0.97730 | 0.97005 | 0.97445 |
| Piece or movement | Suite 1 | 0.99224 | 0.99144 | 0.98835 | 0.98641 | 0.99272 | 0.98976 | 0.99733 | 0.99441 | 0.93554 | 0.99744 | 0.99272 | 0.98976 |
| | Suite 2 | 0.99323 | 0.99578 | 0.99168 | 0.99395 | 0.99328 | 0.99681 | 0.97859 | 0.99863 | 0.99781 | 0.99503 | 0.99328 | 0.99681 |
| | Mozart sonata | 0.98566 | 0.99485 | 0.99137 | 0.97616 | 0.99842 | 0.95533 | 0.86825 | 0.99834 | 0.97652 | 0.80946 | 0.99842 | 0.95533 |
| | First mov. Partita | 0.99620 | 0.99487 | 0.99018 | 0.99331 | 0.99342 | 0.99729 | 0.96832 | 0.99709 | 0.92956 | 0.98097 | 0.99342 | 0.99729 |
| | Piccolo concerto | 0.99132 | 0.99408 | 0.99283 | 0.99295 | 0.98227 | 0.98902 | 0.91862 | 0.96318 | 0.93085 | 0.97725 | 0.98227 | 0.98902 |
| | **Average** | **0.99** | **0.99** | **0.99** | **0.98** | **0.99** | **0.99** | **0.96** | **0.97** | **0.98** | **0.97** | **0.99** | **0.99** |
| | **Standard deviation** | **0.01** | **0.01** | **0.00** | **0.01** | **0.00** | **0.01** | **0.06** | **0.05** | **0.03** | **0.05** | **0.01** | **0.02** |

**Supplementary Table 2. Determination coefficient $R^2$ for the fit to an exponential function of the Complementary Cumulative Distribution Functions (CCDF) and histograms.** For the CCDF, the exponential functions are in the form: $P(x) = A_{\pm}e^{-|x|/B_{\pm}}$, and for histograms $P(X) = C_{\pm}e^{-|X|/D_{\pm}}$. Ascending transitions are identified by the sign "+", descending transitions are identified by the sign "-", and their combination is left without sign. We have used the notation $x$ and $X$ to distinguish between CCDF and histograms (constructed over bins) respectively; in both cases, this notation applies to the quantities $f_j - f_i$ and $f_j^2 - f_i^2$. $A_{\pm}$, $B_{\pm}$, $C_{\pm}$, and $D_{\pm}$ are reported in Supplementary Table 4 (".xlsx" file).

## Comparison in histograms between a random melodic line and the bin degeneracy distribution

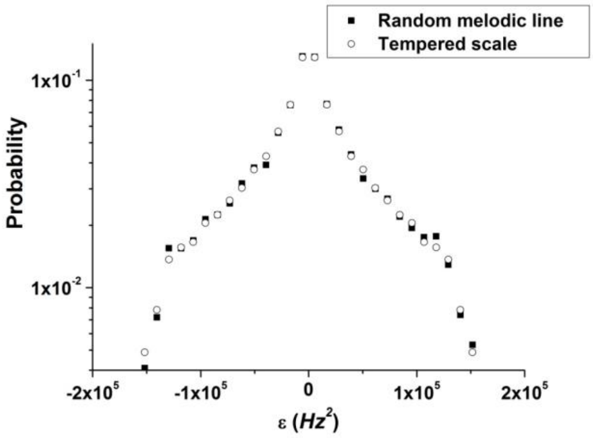


**Supplementary Figure 2. Comparison between histograms for a random melodic line played in the twelve-tone equal-tempered scale (*A*=440 *Hz*) and the bin degeneracy for the same scale.** The random melodic line contains 10000 pitches without rests (9999 transitions) and was generated in the same *ambitus* as the *Suite No. 1 in G Major BWV 1007* by Johann Sebastian Bach (65.406 *Hz* – 391.995 *Hz*). The bin width, 11242 $Hz^2$, is given by Sturges criterion.

## Determination coefficient $R^2$ for the fit of the bin degeneracy distribution to a power law and an exponential function

| | | Twelve-tone equal-tempered scale | | | |
|---|---|---|---|---|---|
| | | Exponential | Power law: $P = a\,(\varepsilon^b)$ | | |
| | | $R^2$ | $R^2$ | $a$ | $b$ $(Hz^2)$ |
| Third Brandenbug Concerto | Violin 1 + | 0.9026 | 0.9792 | 123.9960 ± 31.5998 | -0.6499 ± 0.0221 |
| | Violin 1 - | 0.9026 | 0.9792 | 123.9960 ± 31.5998 | -0.6499 ± 0.0221 |
| | Violin 2 + | 0.9145 | 0.9753 | 136.9747 ± 41.1827 | -0.6538 ± 0.0261 |
| | Violin 2 - | 0.9145 | 0.9753 | 136.9747 ± 41.1827 | -0.6538 ± 0.0261 |
| | Violin 3 + | 0.9080 | 0.9771 | 161.9699 ± 48.1685 | -0.6688 ± 0.0259 |
| | Violin 3 - | 0.9080 | 0.9771 | 161.9699 ± 48.1685 | -0.6688 ± 0.0259 |
| | Viola 1 + | 0.9232 | 0.9656 | 34.2822 ± 9.6377 | -0.5986 ± 0.0266 |
| | Viola 1 - | 0.9232 | 0.9656 | 34.2822 ± 9.6377 | -0.5986 ± 0.0266 |
| | Viola 2 + | 0.9275 | 0.9637 | 39.7147 ± 12.5493 | -0.6066 ± 0.0301 |
| | Viola 2 - | 0.9275 | 0.9637 | 39.7147 ± 12.5493 | -0.6066 ± 0.0301 |
| | Viola 3 + | 0.9263 | 0.9644 | 44.0636 ± 13.5940 | -0.6203 ± 0.0295 |
| | Viola 3 - | 0.9263 | 0.9644 | 44.0636 ± 13.5940 | -0.6203 ± 0.0295 |
| | Cello 1 + | 0.9708 | 0.9712 | 33.0657 ± 10.1810 | -0.6501 ± 0.0336 |
| | Cello 1 - | 0.9708 | 0.9712 | 33.0657 ± 10.1810 | -0.6501 ± 1.0336 |
| | Cello 2 + | 0.9708 | 0.9712 | 33.3237 ± 10.2737 | -0.6501 ± 0.0336 |
| | Cello 2 - | 0.9708 | 0.9712 | 33.3237 ± 10.2737 | -0.6501 ± 1.0336 |
| | Cello 3 + | 0.9708 | 0.9712 | 33.0734 ± 10.1837 | -0.6501 ± 0.0336 |
| | Cello 3 - | 0.9708 | 0.9712 | 33.0734 ± 10.1837 | -0.6501 ± 1.0336 |
| | Violone + | 0.9349 | 0.9691 | 11.8566 ± 3.0126 | -0.6439 ± 0.0327 |
| | Violone - | 0.9349 | 0.9691 | 12.8566 ± 3.0126 | -0.6439 ± 1.0327 |
| | Harpsichord + | 0.9349 | 0.9691 | 28.9525 ± 8.6596 | -0.6439 ± 0.0327 |
| | Harpsichord - | 0.9349 | 0.9691 | 29.9525 ± 8.6596 | -0.6439 ± 1.0327 |
| Missa Dixit Maria | Soprano + | 0.9308 | 0.9334 | 10.6983 ± 3.3090 | -0.5109 ± 0.0291 |
| | Soprano - | 0.9308 | 0.9334 | 10.6983 ± 3.3090 | -0.5109 ± 0.0291 |
| | Contralto + | 0.9536 | 0.9332 | 9.9610 ± 3.2279 | -0.5201 ± 0.0320 |
| | Contralto - | 0.9536 | 0.9332 | 9.9610 ± 3.2279 | -0.5201 ± 0.0320 |
| | Tenor + | 0.9505 | 0.9064 | 7.0496 ± 2.9177 | -0.5059 ± 0.0442 |
| | Tenor - | 0.9505 | 0.9064 | 7.0496 ± 2.9177 | -0.5059 ± 0.0442 |
| | Bass + | 0.9536 | 0.9344 | 6.3891 ± 1.9304 | -0.5294 ± 0.0336 |
| | Bass - | 0.9536 | 0.9344 | 6.3891 ± 1.9304 | -0.5294 ± 0.0336 |
| Piece or movement | Suite 1 + | 0.9709 | 0.9811 | 50.5223 ± 12.9044 | -0.6772 ± 0.0271 |
| | Suite 1 - | 0.9709 | 0.9811 | 50.5223 ± 12.9044 | -0.6772 ± 0.0271 |
| | Suite 2 + | 0.9099 | 0.9778 | 27.1223 ± 6.0524 | -0.6385 ± 0.0239 |
| | Suite 2 - | 0.9099 | 0.9778 | 27.1223 ± 6.0524 | -0.6385 ± 0.0239 |
| | Mozart sonata + | 0.8488 | 0.9831 | 140.7220 ± 23.7195 | -0.6662 ± 0.0142 |
| | Mozart sonata - | 0.8488 | 0.9831 | 140.7220 ± 23.7195 | -0.6662 ± 0.0142 |
| | First mov. Partita + | 0.8966 | 0.9736 | 123.9510 ± 33.5126 | -0.6241 ± 0.0221 |
| | First mov. Partita - | 0.8966 | 0.9736 | 123.9510 ± 33.5126 | -0.6241 ± 0.0221 |
| | Piccolo concerto + | 0.9724 | 0.9626 | 275.1436 ± 129.9877 | -0.6052 ± 0.0350 |
| | Piccolo concerto - | 0.9724 | 0.9626 | 275.1436 ± 129.9877 | -0.6052 ± 0.0350 |
| | **Average** | **0.934** | **0.963** | | |

**Supplementary Table 3. Functional form of the “degeneracy” probability distribution for the twelve-tone equal-tempered scale.** Determination coefficient $R^2$ for the fit to exponential and power law functions of the “degeneracy” distribution.

# Relation between the bin center and the average of the possible transitions $f_j^2 - f_i^2$ inside the bin for a typical case

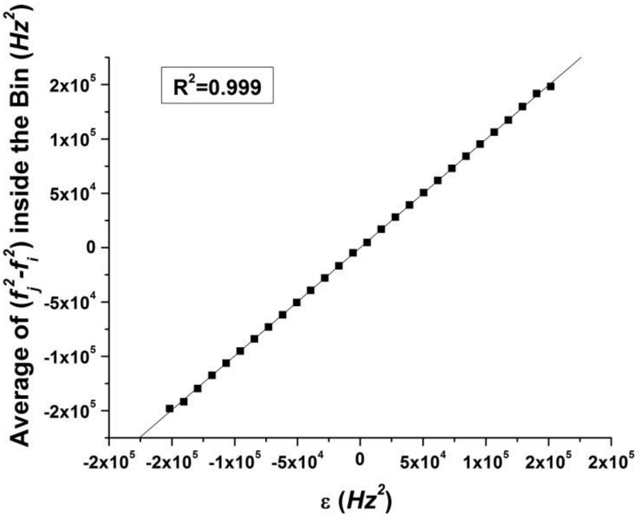


**Supplementary Figure 3. Relation between the bin center and the average of the possible transitions $f_j^2 - f_i^2$ inside the bin.**

The fit shows a lineal relation of the form $\overline{f_j^2 - f_i^2} = A + B\varepsilon$ with $A = -8.315 \times 10^{-12} \pm 195.370$, $B = 0.996 \pm 0.002$ and determination coefficient $R^2 = 0.999$. Since $A$ and $B$ are close to 0 and 1, respectively, then the number associated with each bin center is representative of the possible transitions $f_j^2 - f_i^2$ inside the bin. Bin width 11242 $Hz^2$, *ambitus* 65.406 $Hz$ to 391.995 $Hz$.

# Calculation details for the quantity $\langle|\varepsilon|\rangle$

Assuming that each bin can be represented by the average of its extremes (Supplementary Figure 3 shows a typical case), and this number corresponds to the average of all possible states in the bin $\left[\overline{(f_j^2 - f_i^2)}\right]_k$ generated from the corresponding *ambitus*, then we can link the quantities $\langle|\varepsilon|\rangle$ and $f_j^2 - f_i^2$ and measure the expected value as

$$\langle|\varepsilon|\rangle = \sum_{k=1}^{N}\left[p_k \cdot \left(\left[\overline{|f_j^2 - f_i^2|}\right]_k\right)\right].$$

This last equation depends on the quantity $\left[\overline{|f_j^2 - f_i^2|}\right]_k$, which can be calculated for each bin from the relation $f_j + f_i = (-1)^h\, a\, L^{-b}\, (f_j - f_i)$, employing the fact that $f_j^2 - f_i^2 = (f_j + f_i)(f_j - f_i)$. Then

$$\left[\overline{|f_j^2 - f_i^2|}\right]_k = \frac{1}{n_k}\sum_{u=1}^{n_k}|f_j^2 - f_i^2|_u = \frac{1}{n_k}\sum_{u=1}^{n_k} a\, L^{-b}(f_j - f_i)_u^2$$

where the sum varies from $u = 1$ to the total number of possible transitions $f_j^2 - f_i^2$ in the $k^{th}$ bin, $u = n_k$. Since there are different combinations of pairs of frequencies that generate the same size of interval , we can split the sum into as many terms as possible for interval sizes inside the bin

$$\left[\overline{|f_j^2 - f_i^2|}\right]_k = \frac{a}{n_k}\sum_{x=1}^{W}\left[\frac{n_x}{n_x}L_x^{-b}\sum_x (f_i - f_i)_x^2\right] = a\sum_{x=1}^{W}\left\{\frac{n_x}{n_k}L_x^{-b}\left[\frac{1}{n_x}\sum_x (f_i - f_i)_x^2\right]\right\} = a\sum_{x=1}^{W}\left[\mathcal{P}(x)L_x^{-b}\,\overline{(f_i - f_i)^2}_x\right],$$

where $n(x)$ refers to the total number of intervals of size $x$ inside the bin. The sum of all possible transitions (inside the bin) is expressed as a sum of all possible interval sizes inside it. In this last equation, the sum varies from $x = 1$ to the maximum interval size in the $k^{th}$ bin, $x = W$.

$\mathcal{P}(x)$ is the probability of finding an interval of size $x$ inside the $k^{th}$ bin, and $\overline{(f_j - f_i)^2}_x$ is the average of the quantity $(f_j - f_i)^2$ for intervals of size $x$ inside the bin.

The quantity $\overline{(f_j - f_i)^2}_x$ can be related to the tonal consonance parameter $f_i - f_i$ over a single interval size $x$ expressing it as $\sigma_x^2 + \overline{|f_j - f_i|}_x^2$, where $\sigma_x^2$ is a variance that we can associate with the spreading of forms used to construct a single kind of interval of size $x$ in the $k^{th}$ bin and $\overline{|f_j - f_i|}_x^2$ depends on the average of the absolute value for the frequency differences of a single interval size $x$. Then

$$\left[\overline{|f_j^2 - f_i^2|}\right]_k = a\sum_{x=1}^{W}\left\{\mathcal{P}(x)L_x^{-b}\,\left[\sigma_x^2 + \overline{|f_j - f_i|}_x^2\right]\right\} = a\sum_{x=1}^{W}\left[\mathcal{P}(x)L_x^{-b}\,\sigma_x^2\right] + a\sum_{x=1}^{W}\left[\mathcal{P}(x)L_x^{-b}\,\overline{|f_j - f_i|}_x^2\right]$$

Taking $b \cong 1$ and using the notation $\langle{}^{\sigma^2}/_{L}\rangle_k$ and $\langle\overline{|f_j - f_i|}^2/L\,\rangle_k$ to represent the corresponding expected values inside each bin

$$\left[\overline{|f_j^2 - f_i^2|}\right]_k = a\,\langle \sigma^2/_L \rangle_k + a\,\langle \overline{|f_j - f_i|}^2/L\,\rangle_k$$

Since the expected value operator $E$ is linear and each bin is characterized by the sum of two quantities, $a\,\langle \sigma^2/_L \rangle_k \equiv X$ and $a\,\langle \overline{|f_j - f_i|}^2/L\,\rangle_k \equiv Y$, then the expected value of all bins is $E(X+Y) = E(X) + E(Y)$, showing that

$$\langle|\varepsilon|\rangle \;= a\sum_{k=1}^{N} p_k\,\langle \sigma^2/_L \rangle_k + a\sum_{k=1}^{N} p_k\,\langle \overline{|f_j - f_i|}^2/L\,\rangle_k$$

## Relating the average of the quantity $\overline{|f_j - f_i|}$ to an average of tonal consonance

If we consider a certain interval of size $L$ and we move it in the register, then the frequency difference $|f_j - f_i|$ is a soft function $F$ of the tonal consonance, measured through a level of dissonance "$D$". Since inside a bin the frequency differences of the same interval size are near each other, then we can approximate the relation between tonal consonance and frequency difference around a point $q$ using the Taylor series

$$|f_j - f_i| = F(D) \approx F(q) + F'(q)D - F'(q)q.$$

Taking the mean value of the $M$ frequency differences of the same size *x* inside the bin

$$\overline{|f_j - f_i|} = \frac{1}{M}\sum_{U=1}^{M}|f_j - f_i|_U = \frac{1}{M}\sum_{U=1}^{M}F(D)_U \approx F(q)\frac{1}{M}\sum_{U=1}^{M}1 + F'(q)\frac{1}{M}\sum_{U=1}^{M}D_U - F'(q)q\frac{1}{M}\sum_{U=1}^{M}1,$$

and taking $q$ as the mean value of the dissonance level corresponding to the $M$ frequency differences of the same size inside the bin: $q = \bar{D} = \frac{1}{M}\sum_{U=1}^{M} D_U$ then

$$\overline{|f_j - f_i|} \approx F(\bar{D}) + F'(\bar{D})\bar{D} - F'(\bar{D})\bar{D} = F(\bar{D}).$$

This result implies that the average of the frequency differences corresponds to the frequency difference that is representative of the corresponding average of tonal consonance.

## Minimization of the relative entropy subject to constraints

In order to carry out the optimization of the quantity $D_{KL} = \sum_{n=1}^{N} p_n \ln\left(\frac{p_n}{q_n}\right)$ subject to constraints, we used the Lagrange multipliers method.

In this method, we have a function $f(p_1, p_2, \dots, p_N)$ for which we want to know its extremes subject to the "$l$" constraints:

$g_1(p_1, p_2, \dots, p_N) = 0,\; g_2(p_1, p_2, \dots, p_N) = 0, \dots,\; g_l(p_1, p_2, \dots, p_N) = 0.$

In our case:

$f(p_1, p_2, \dots, p_N) = \sum_{n=1}^{N} p_n \ln\left(\frac{p_n}{q_n}\right)$

$$g_1(p_1, p_2, \dots, p_N) = \sum_{n=1}^{\frac{N}{2}} p_n - (p_d + p_u) = 0$$

$$g_2(p_1, p_2, \dots, p_N) = \sum_{n=\frac{N}{2}+1}^{N} p_n - (p_a + p_u) = 0$$

$g_3(p_1, p_2, \dots, p_N) = \sum_{n=1}^{N} p_n|\varepsilon_n| - < |\varepsilon| >= 0$

$g_4(p_1, p_2, \dots, p_N) = \sum_{n=1}^{N} p_n\varepsilon_n - < \varepsilon >= 0$

Then we construct the auxiliary function $L$ containing the Lagrange multipliers (one per constraint):

$$L(p_1, p_2, \dots, p_N, \lambda_-, \lambda_+, \lambda_1, \lambda_2) = f(p_1, p_2, \dots, p_N) + (\lambda_-)g_1(p_1, p_2, \dots, p_N) + (\lambda_+)g_2(p_1, p_2, \dots, p_N) + (\lambda_1)g_3(p_1, p_2, \dots, p_N) + (\lambda_2)g_4(p_1, p_2, \dots, p_N)$$

In order to find the extremes, we have to solve the equations system:

$$\frac{\partial L}{\partial p_n} = 0\,,(n \in [1,N])\,;\; \frac{\partial L}{\partial \lambda_-} = 0\,;\; \frac{\partial L}{\partial \lambda_+} = 0\,;\; \frac{\partial L}{\partial \lambda_1} = 0\,;\; \frac{\partial L}{\partial \lambda_2} = 0$$

In the case of the derivatives with respect to the Lagrange multipliers we obtain the constraints:

$$\frac{\partial L}{\partial \lambda_-} = g_1(p_1, p_2, \dots, p_N) = 0\ ;\ \frac{\partial L}{\partial \lambda_+} = g_2(p_1, p_2, \dots, p_N) = 0\ ;\ \frac{\partial L}{\partial \lambda_1} = g_3(p_1, p_2, \dots, p_N) = 0\ ;\ \frac{\partial L}{\partial \lambda_2} = g_4(p_1, p_2, \dots, p_N) = 0$$

In the case of $\frac{\partial L}{\partial p_n} = 0$ we have:

$$L = \sum_{n=1}^{N} p_n \ln\left(\frac{p_n}{q_n}\right) + \lambda_-\left(\sum_{n=1}^{\frac{N}{2}} p_n - (p_d + p_u)\right) + \lambda_+\left(\sum_{n=\frac{N}{2}+1}^{N} p_n - (p_a + p_u)\right) + \lambda_1\left(\sum_{n=1}^{N} p_n|\varepsilon_n| - <|\varepsilon|>\right) + \lambda_2\left(\sum_{n=1}^{N} p_n\varepsilon_n - <\varepsilon>\right)$$

$$\Rightarrow L = \sum_{n=1}^{N}\left[p_n \ln\left(\frac{p_n}{q_n}\right) + \lambda_1 p_n|\varepsilon_n| + \lambda_2 p_n \varepsilon_n\right] + \lambda_- \sum_{n=1}^{\frac{N}{2}} p_n + \lambda_+ \sum_{n=\frac{N}{2}+1}^{N} p_n - \lambda_-(p_d + p_u) - \lambda_+(p_a + p_u) - \lambda_1 <|\varepsilon|> - \lambda_2 <\varepsilon>$$

Then, for $n \in [1, N/2]$

$$\frac{\partial L}{\partial p_n} = \ln\left(\frac{p_n}{q_n}\right) + \frac{q_n}{p_n}\cdot\frac{p_n}{q_n} + \lambda_1|\varepsilon_n| + \lambda_2\varepsilon_n + \lambda_- = \ln\left(\frac{p_n}{q_n}\right) + \lambda_1|\varepsilon_n| + \lambda_2\varepsilon_n + \lambda_-^* = 0\ \text{, with } \lambda_-^* = 1 + \lambda_-$$

and for $n \in \left[\left(\frac{N}{2}\right) + 1, N\right]$

$$\frac{\partial L}{\partial p_n} = \ln\left(\frac{p_n}{q_n}\right) + \frac{q_n}{p_n}\cdot\frac{p_n}{q_n} + \lambda_1|\varepsilon_n| + \lambda_2\varepsilon_n + \lambda_+ = \ln\left(\frac{p_n}{q_n}\right) + \lambda_1|\varepsilon_n| + \lambda_2\varepsilon_n + \lambda_+^* = 0\ \text{, with } \lambda_+^* = 1 + \lambda_-$$

Solving, we have:

$$p_n = \begin{cases} q_n \cdot \exp(-\lambda_1|\varepsilon_n| - \lambda_2\varepsilon_n - \lambda_-^*) \text{ for } n \in \left[1, \frac{N}{2}\right] \\ q_n \cdot \exp(-\lambda_1|\varepsilon_n| - \lambda_2\varepsilon_n - \lambda_+^*) \text{ for } n \in \left[\frac{N}{2} + 1, N\right] \end{cases}$$

Using the constraints $g_1(p_1, p_2, \dots, p_N)$ and $g_2(p_1, p_2, \dots, p_N)$, we can deduce the quantities $\exp(-\lambda_-^*)$ and $\exp(-\lambda_+^*)$

$$\sum_{n=1}^{\frac{N}{2}} q_n \cdot \exp(-\lambda_-^*) \cdot \exp(-\lambda_1|\varepsilon_n| - \lambda_2\varepsilon_n) = p_d + p_u \Rightarrow \exp(-\lambda_-^*) = \frac{p_d + p_u}{\sum_{n=1}^{\frac{N}{2}} q_n \cdot \exp(-\lambda_1|\varepsilon_n| - \lambda_2\varepsilon_n)} \text{ for } n \in \left[1, \frac{N}{2}\right],$$

$$\sum_{n=\frac{N}{2}+1}^{N} q_n \cdot \exp(-\lambda_+^*) \cdot \exp(-\lambda_1|\varepsilon_n| - \lambda_2\varepsilon_n) = p_a + p_u \Rightarrow \exp(-\lambda_+^*) = \frac{p_a + p_u}{\sum_{n=\frac{N}{2}+1}^{N} q_n \cdot \exp(-\lambda_1|\varepsilon_n| - \lambda_2\varepsilon_n)} \text{ for } n \in \left[\frac{N}{2} + 1, N\right]$$

Finally, the probabilities $p_n$ are given by

$$p_n = \begin{cases} \dfrac{q_n \cdot (p_d + p_u) \cdot \exp(-\lambda_1|\varepsilon_n| - \lambda_2\varepsilon_n)}{\sum_{n=1}^{\frac{N}{2}}[q_n \cdot \exp(-\lambda_1|\varepsilon_n| - \lambda_2\varepsilon_n)]} \text{ for } n \in \left[1, \frac{N}{2}\right] \\ \dfrac{q_n \cdot (p_a + p_u) \cdot \exp(-\lambda_1|\varepsilon_n| - \lambda_2\varepsilon_n)}{\sum_{n=(N/2+1)}^{N}[q_n \cdot \exp(-\lambda_1|\varepsilon_n| - \lambda_2\varepsilon_n)]} \text{ for } n \in \left[\frac{N}{2} + 1, N\right] \end{cases}$$

Now, in order to prove that our solution $p_n$ corresponds to a minimum, we suppose that there is another possible solution $\mathrm{P}_n$ that also satisfies the constraints, that is:

$$\sum_{n=1}^{\frac{N}{2}} p_n = \sum_{n=1}^{\frac{N}{2}} \mathrm{P}_n = p_d + p_u$$

$$\sum_{n=\frac{N}{2}+1}^{N} p_n = \sum_{n=\frac{N}{2}+1}^{N} \mathrm{P}_n = p_a + p_u$$

$$\sum_{n=1}^{N} p_n|\varepsilon_n| = \sum_{n=1}^{N} \mathrm{P}_n|\varepsilon_n| = < |\varepsilon| >$$

$$\sum_{n=1}^{N} p_n\varepsilon_n = \sum_{n=1}^{N} \mathrm{P}_n\varepsilon_n =< \varepsilon >$$

The relative entropies associated with $p_n$ and $\mathrm{P}_n$ are:

$$D_{KL}(p_n|q_n) = \sum_{n=1}^{N} p_n \ln\left(\frac{p_n}{q_n}\right) \qquad ; \qquad D_{KL}(\mathrm{P}_n|q_n) = \sum_{n=1}^{N} \mathrm{P}_n \ln\left(\frac{\mathrm{P}_n}{q_n}\right)$$

Next, if we show that the quantity $D_{KL}(\mathrm{P}_n|q_n) - D_{KL}(p_n|q_n)$ is always greater or equal to 0 for all possible $\mathrm{P}_n$ that satisfy the constraints, then $p_n$ is a minimum.

$$\Longrightarrow D_{KL}(\mathrm{P}_n|q_n) - D_{KL}(p_n|q_n) = \sum_{n=1}^{N} \mathrm{P}_n \ln\left(\frac{\mathrm{P}_n}{q_n}\right) - \sum_{n=1}^{N} p_n \ln\left(\frac{p_n}{q_n}\right) = \sum_{n=1}^{N} \mathrm{P}_n \ln\left(\frac{\mathrm{P}_n}{q_n}\right) - \left[\sum_{n=1}^{N/2} p_n \ln\left(\frac{p_n}{q_n}\right) + \sum_{n=\frac{N}{2}+1}^{N} p_n \ln\left(\frac{p_n}{q_n}\right)\right]$$

As:

$$p_n = \begin{cases} q_n \cdot \exp(-\lambda_1|\varepsilon_n| - \lambda_2\varepsilon_n - \lambda_-^*) \text{ for } n \in \left[1, \frac{N}{2}\right] \\ q_n \cdot \exp(-\lambda_1|\varepsilon_n| - \lambda_2\varepsilon_n - \lambda_+^*) \text{ for } n \in \left[\frac{N}{2}+1, N\right] \end{cases}$$

Then:

$$\ln\left(\frac{p_n}{q_n}\right) = \begin{cases} (-\lambda_1|\varepsilon_n| - \lambda_2\varepsilon_n - \lambda_-^*) \text{ for } n \in \left[1, \frac{N}{2}\right] \\ (-\lambda_1|\varepsilon_n| - \lambda_2\varepsilon_n - \lambda_+^*) \text{ for } n \in \left[\frac{N}{2}+1, N\right] \end{cases}$$

Thus:

$$D_{KL}(\mathrm{P}_n|q_n) - D_{KL}(p_n|q_n) = \sum_{n=1}^{N} \mathrm{P}_n \ln\left(\frac{\mathrm{P}_n}{q_n}\right) - \left[\sum_{n=1}^{N/2} p_n\,(-\lambda_1|\varepsilon_n| - \lambda_2\varepsilon_n - \lambda_-^*) + \sum_{n=\frac{N}{2}+1}^{N} p_n(-\lambda_1|\varepsilon_n| - \lambda_2\varepsilon_n - \lambda_+^*)\right]$$

$$= \sum_{n=1}^{N} \mathrm{P}_n \ln\left(\frac{\mathrm{P}_n}{q_n}\right) - \left[-\lambda_-^* \sum_{n=1}^{N/2} p_n - \lambda_1 \sum_{n=1}^{N/2} p_n\,|\varepsilon_n| - \lambda_2 \sum_{n=1}^{N/2} p_n\,\varepsilon_n - \lambda_+^* \sum_{n=\frac{N}{2}+1}^{N} p_n - \lambda_1 \sum_{n=\frac{N}{2}+1}^{N} p_n\,|\varepsilon_n| - \lambda_2 \sum_{n=\frac{N}{2}+1}^{N} p_n\,\varepsilon_n\right]$$

$$= \sum_{n=1}^{N} \mathrm{P}_n \ln\left(\frac{\mathrm{P}_n}{q_n}\right) -\!- \lambda_-^* \sum_{n=1}^{\frac{N}{2}} p_n - \lambda_+^* \sum_{n=\frac{N}{2}+1}^{N} p_n - \lambda_1 \sum_{n=1}^{N} p_n\,|\varepsilon_n| - \lambda_2 \sum_{n=1}^{N} p_n\,\varepsilon_n$$

$$= \sum_{n=1}^{N} \mathrm{P}_n \ln\left(\frac{\mathrm{P}_n}{q_n}\right) - [-\lambda_-^*(p_d + p_u) - \lambda_+^*(p_a + p_u) - \lambda_1 < |\varepsilon| > -\lambda_2 < \varepsilon >]$$

Since $p_n$ and $\mathrm{P}_n$ satisfy the constraints, then:

$$D_{KL}(\mathrm{P}_n|q_n) - D_{KL}(p_n|q_n) = \sum_{n=1}^{N} \mathrm{P}_n \ln\left(\frac{\mathrm{P}_n}{q_n}\right) - \left[-\lambda_-^* \sum_{n=1}^{N/2} \mathrm{P}_n - \lambda_+^* \sum_{n=\frac{N}{2}+1}^{N} \mathrm{P}_n - \lambda_1 \sum_{n=1}^{N} \mathrm{P}_n\,|\varepsilon_n| - \lambda_2 \sum_{n=1}^{N} \mathrm{P}_n\,\varepsilon_n\right]$$

$$= \sum_{n=1}^{N} \mathrm{P}_n \ln\left(\frac{\mathrm{P}_n}{q_n}\right) - \left[ -\lambda_-^* \sum_{n=1}^{N/2} \mathrm{P}_n - \lambda_+^* \sum_{n=\frac{N}{2}+1}^{N} \mathrm{P}_n - \lambda_1 \sum_{n=1}^{N/2} \mathrm{P}_n\, |\varepsilon_n| - \lambda_2 \sum_{n=1}^{N/2} \mathrm{P}_n\, \varepsilon_n - \lambda_1 \sum_{n=\frac{N}{2}+1}^{N} \mathrm{P}_n\, |\varepsilon_n| - \lambda_2 \sum_{n=\frac{N}{2}+1}^{N} \mathrm{P}_n\, \varepsilon_n \right]$$

$$= \sum_{n=1}^{N} \mathrm{P}_n \ln\left(\frac{\mathrm{P}_n}{q_n}\right) - \left[ \sum_{n=1}^{N/2} \mathrm{P}_n\, (-\lambda_1|\varepsilon_n| - \lambda_2\varepsilon_n - \lambda_-^*) + \sum_{n=\frac{N}{2}+1}^{N} \mathrm{P}_n(-\lambda_1|\varepsilon_n| - \lambda_2\varepsilon_n - \lambda_+^*) \right]$$

$$= \sum_{n=1}^{N} \left[ \mathrm{P}_n \ln\left(\frac{\mathrm{P}_n}{q_n}\right)\right] - \sum_{n=1}^{N} \left[ \mathrm{P}_n \ln\left(\frac{p_n}{q_n}\right)\right] = \sum_{n=1}^{N} \left[ \mathrm{P}_n \ln\left(\frac{\mathrm{P}_n}{q_n}\right) - \ln\left(\frac{p_n}{q_n}\right)\right] = \sum_{n=1}^{N} \left[ \mathrm{P}_n \ln\left(\frac{\mathrm{P}_n}{p_n}\right)\right]$$

Now, since $\mathrm{P}_n$ and $p_n$ don't satisfy the normalization constraint ($p_d + p_u + p_a = 1$), then we can construct $\mathrm{P}_n^*$ and $p_n^*$ multiplying $\mathrm{P}_n$ and $p_n$ by a constant factor:

$$\sum_{n=1}^{N} \mathrm{P}_n = \sum_{n=1}^{N} p_n = p_d + 2p_u + p_a = 1 + p_u$$

$$\Rightarrow \mathrm{P}_n^* = \frac{\mathrm{P}_n}{1+p_u} \ ; p_n^* = \frac{p_n}{1+p_u}$$

$$\Rightarrow \sum_{n=1}^{N} \mathrm{P}_n^* = \sum_{n=1}^{N} p_n^* = 1$$

Thus:

$$D_{KL}(\mathrm{P}_n|q_n) - D_{KL}(p_n|q_n) = (1+p_u) \sum_{n=1}^{N} \frac{\mathrm{P}_n}{1+p_u} \ln\left( \frac{\mathrm{P}_n \cdot \frac{1}{1+p_u}}{p_n \cdot \frac{1}{1+p_u}} \right) = (1+p_u) \sum_{n=1}^{N} \left[ \mathrm{P}_n^* \ln\left(\frac{\mathrm{P}_n^*}{p_n^*}\right)\right],$$

and as the relative entropy $\sum_{n=1}^{N} \left[ \mathrm{P}_n^* \ln\left(\frac{\mathrm{P}_n^*}{p_n^*}\right)\right]$ is always greater or equal to 0 (equal to 0 only in the case $\mathrm{P}_n^* = p_n^*$) and $(1+p_u) \geq 1$, then

$$D_{KL}(\mathrm{P}_n|q_n) - D_{KL}(p_n|q_n) \geq 0 \ ,$$

showing that $p_n$ corresponds to a minimum.

Note that using the normalized probability conditions in the minimization problem:

$$\sum_{n=1}^{\frac{N}{2}} p_n^* = \frac{(p_d + p_u)}{1+p_u} \qquad \text{and} \qquad \sum_{n=\frac{N}{2}+1}^{N} p_n^* = \frac{(p_a + p_u)}{1+p_u},$$

instead of the constraints $g_1$ and $g_2$, the result of the minimization problem (using $p_n^*$ instead of $p_n$) is only changed by the multiplication of a positive constant:

$$p_n^* = \begin{cases} \dfrac{q_n \cdot (p_d + p_u) \cdot \exp(-\lambda_1|\varepsilon_n| - \lambda_2\varepsilon_n)}{(1+p_u)\sum_{n=1}^{\frac{N}{2}}[q_n \cdot \exp(-\lambda_1|\varepsilon_n| - \lambda_2\varepsilon_n)]} \text{for } n \in \left[1, \dfrac{N}{2}\right] \\ \dfrac{q_n \cdot (p_a + p_u) \cdot \exp(-\lambda_1|\varepsilon_n| - \lambda_2\varepsilon_n)}{(1+p_u)\sum_{n=(N/2+1)}^{N}[q_n \cdot \exp(-\lambda_1|\varepsilon_n| - \lambda_2\varepsilon_n)]} \text{ for } n \in \left[\dfrac{N}{2}+1, N\right] \end{cases} .$$

Furthermore, the *a priori* distribution $q_n$ does not change, because if we define $q_n^* = \frac{q_n}{1+p_u'}$, where $p_u'$ is the probability of unisons in the bin degeneracy distribution, the positive constant $\frac{1}{1+p_u'}$ appears in the numerator as well as in the denominator.

## Data, fitting parameters, determination coefficients, expected values, and Lagrange multipliers

This information is presented in the **Supplementary Table 4** contained in the ".xlsx" file attached to the Supplementary Material.
